# Supplementary material for: Direct measurements of air layer profiles under impacting droplets using high-speed color interferometry
Source: arXiv:1111.3762 source file (2011-11-16)
Supplement: Supplementary file 1 [file supplement.pdf]

# Supplemental material: Direct measurements of air layer profiles under impacting droplets using high-speed color interferometry

Van der Veen, Tran*, Lohse and Sun

*t.tran@utwente.nl*

## I. COLOR REPRESENTATION

The sRGB model is generally not preferred when comparing colors between experiments because it does not decouple intensity and color information. In other words, the colors in an interference pattern, if represented by the sRGB model, can be altered due to variation in illumination conditions such as light intensity, incident and observing angles. Instead, we use the CIE 1976 color model (also called CIELAB), a *device–independent* model that is most effective in decoupling light intensity [1].

To assess the importance of decoupling light intensity from color analysis, we present here a test case comparing sRGB and CIELAB models. First we reduce light intensity in the interference pattern resulting from the calibration step by multiplying each channel of the RGB model by 0.75. The darkened pattern is shown in figure 1a. We use this pattern as a color sample from which air layer thickness is recovered. An image showing the color difference using sRGB representation in grayscale between the modified color set and the reference one is shown in figure 1b. Clearly, without intensity decoupling, it is difficult to recover the air thickness profile. Even examining the average color difference along a few candidate profiles does not reveal which one is correct (figure 1d). On the other hand, the color sample after intensity decoupling with CIELAB model gives profiles with high contrast from the background (see figure 1e). Figure 1g also shows that the correct one also has the smallest value of average color difference along candidate profiles in Fig. 1f.

To work with colors in the CIELAB color space, we follow the method described in Ref. [1]: sRGB-format images are converted to an absolute color space (XYZ) and then to CIELAB. A color in CIELAB model has three components: $\boldsymbol{L}$ for lightness information, and $\boldsymbol{a}$ and $\boldsymbol{b}$ for color information. Thus, we can separate light intensity from our analysis by omitting the component $\boldsymbol{L}$. Each reference color $i$ after intensity decoupling is represented

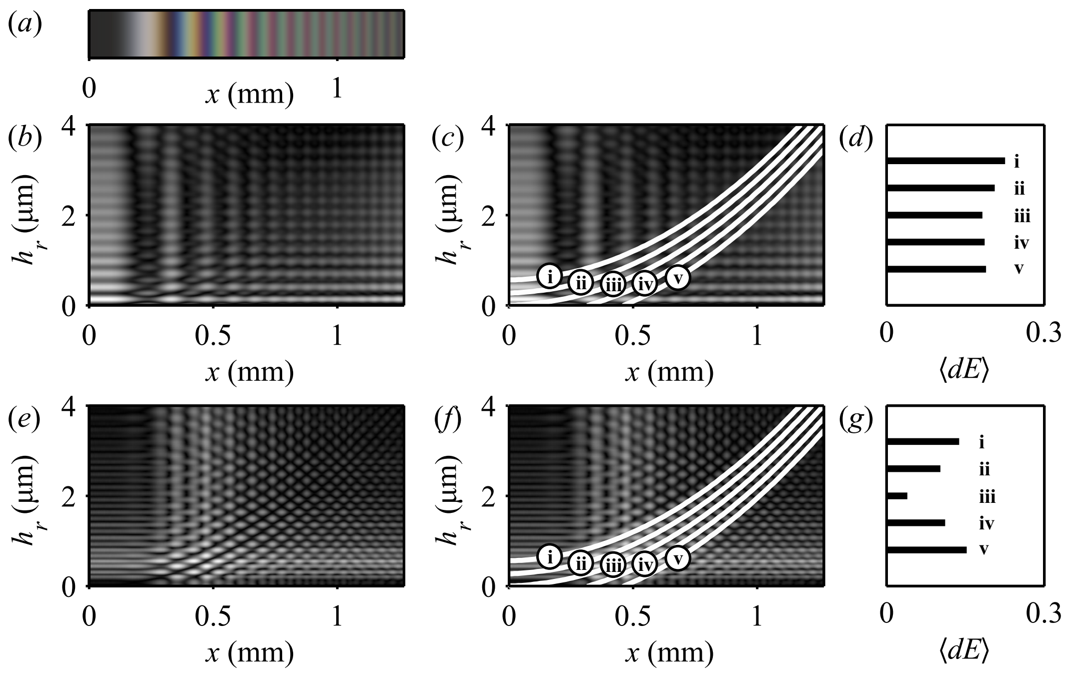


FIG. 1. ($a$) Color variation (after reducing the intensity to 75%) depending on the air film thickness obtained in the calibration step. ($b$) sRGB model: color difference between the reference colors and the darkened ones in grayscale. ($c$) Candidate profiles resulted from the color difference in ($b$). ($d$) The averaged color differences along the candidate profiles shown in ($c$). ($e$) CIELAB model: color difference between the reference colors and the darkened ones in grayscale. ($f$) Candidate profiles resulted from the color difference in ($e$). ($g$) The averaged color differences along the candidate profiles shown in ($f$).

by a two-component vector $(\boldsymbol{a}_r^i, \boldsymbol{b}_r^i)$ and is associated with a value of reference thickness $h_r^i$ for $1 \leq i \leq N$ and $h_r^i$ is in the range $0\,\mu\text{m} \leq h_r \leq 4\,\mu\text{m}$.

We now discuss an inherent issue of methods using color interferometry to measure film thickness regardless of color model, namely, repetition of colors at multiple values of film thickness. Lin & Sullivan [2] used color interferometry to measure thin film thickness and pointed out that the best operating range is from $0.15\,\mu$m to $1\,\mu$m, whereas the range from $0\,\mu$m to $0.15\,\mu$m does not produce truly distinctive colors. We demonstrate this problem for the reference colors represented by CIELAB model in figure 2(a). The plot shows $\boldsymbol{b}_r^i$ vs. $\boldsymbol{a}_r^i$ for $1 \leq i \leq N$ and correspondingly $0 \leq h_r^i \leq 4\,\mu$m. Note that each pair of $(\boldsymbol{a}_r^i, \boldsymbol{b}_r^i)$ represents one color and is associated with a value of thickness $h_r^i$. Thus, at each intersection of the curve with itself, there are two values of thickness producing the same

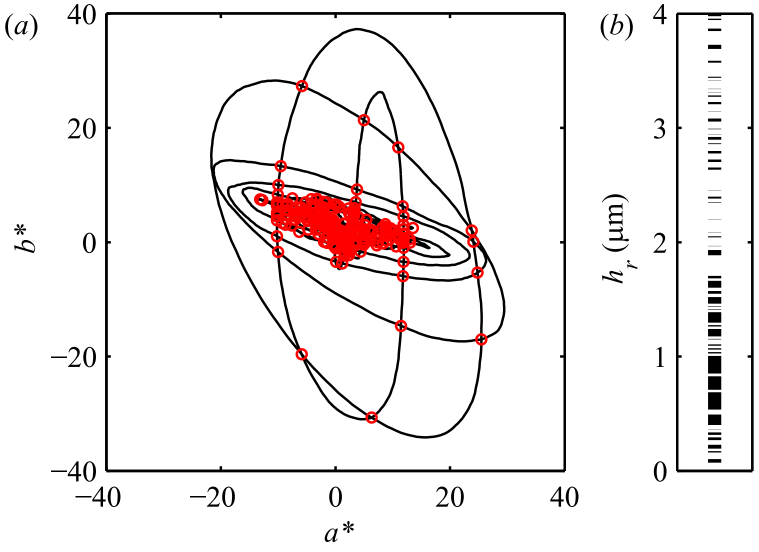


FIG. 2. ($a$) Plot of reference color in $\boldsymbol{a}_r, \boldsymbol{b}_r$ space showing the color is not unique at some thickness values (red circles). ($b$) Only thickness values that have unique color are shown.

color in the interference pattern. By omitting these points, we obtain the thickness values that produce unique colors (figure 2b). It is clearly seen that the color database can be used to estimate film thickness ranging from 0.5 $\mu$m to 1 $\mu$m without ambiguity (note that our range of film thickness for reliable measurements is different from that of [2] because we are using CIELAB model for representing the color). Outside of this range, thickness measurements for individual points are not reliable. The entire profile, however, can be constructed if the smoothness and continuity of thickness profiles are taken into account.

Next, we describe this method for a test case in which we extract the thickness profile of a thin film based on its interference pattern. The film thickness is known in advance and is compared to the computed one to evaluate the method's accuracy.

## II. PROFILE SELECTION AND TEST CASE

First, we generate an interference pattern from an air film between a glass slide and a lens. This arrangement is sketched in figure 3a (the radius of the lens used in this setup is 300 mm, which is different from the one used for calibration). From the resulting interference pattern, we exclude the part where two surfaces are in contact (correspondingly, the color is close to black) to simulate the real situations in which the liquid does not necessarily touch

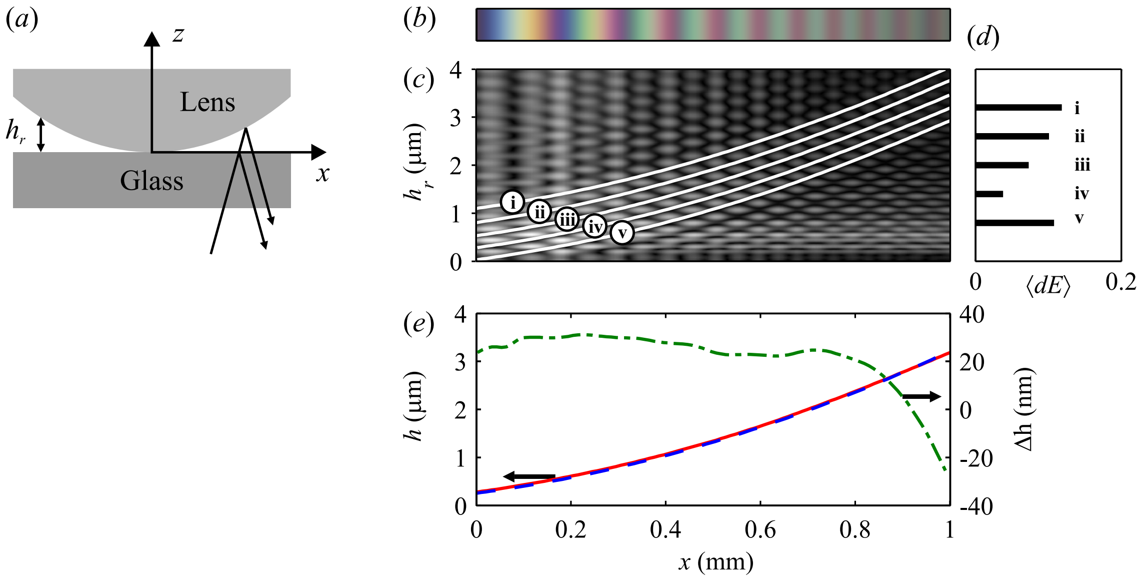


FIG. 3. ($a$) A schematic of the setup for the test case in which a lens (surface radius $R = 300\,\mathrm{mm}$) is placed on top of a glass slide. ($b$) Color sample taken along a radial direction of a interference pattern. The origin $x = 0$ is *not* where the lens and the glass slide are in contact. ($c$) Color difference with candidate profiles in white solid lines. ($d$) Average color difference of candidate profiles shown in ($c$). The selected profile is profile ($iv$). ($e$) Comparison between the selected profile (shown in solid line) and the profile of the lens (shown in dashed line). The difference $\Delta h$ (shown in dashed-dotted line) between the selected profile and the lens's profile.

the solid surface. The film thickness that needs to be determined is within the range of the calibrated thickness. The interference pattern, after average azimuthally and expanded in the transverse direction, is the color sample shown in figure 3b. Note that there is no color variation in the transverse direction and the colors are converted to CIELAB color space for analysis. Thus, in the $x$ direction, the number of pixels is $M = 1737$; each pixel has coordinate $x_j$ and a color represented by a vector $(\boldsymbol{a}_e^j, \boldsymbol{b}_e^j)$ for $1 \le j \le M$.

For each color in the sample $(\boldsymbol{a}_e^j, \boldsymbol{b}_e^j)$ and each reference color $(\boldsymbol{a}_r^i, \boldsymbol{b}_r^i)$, we can calculate the color difference using the Euclidean distance:

$$dE^{ij} = \left[(\boldsymbol{a}_e^j - \boldsymbol{a}_r^i)^2 + (\boldsymbol{b}_e^j - \boldsymbol{b}_r^i)^2\right]^{1/2} \quad \text{for} \quad 1 \le i \le N,\, 1 \le j \le M. \tag{1}$$

Since each color $(\boldsymbol{a}_e^j, \boldsymbol{b}_e^j)$ is associated with a coordinate $x_j$ and, recall that each reference color $(\boldsymbol{a}_r^i, \boldsymbol{b}_r^i)$ is associated with a value of reference thickness $h_r^i$, the color difference $dE^{ij}$

can be thought of as a function of $h_r^i$ and $x_j$:

$$dE^{ij} = f\left(h_r^i, x_j\right) \quad \text{for} \quad 1 \le i \le N,\, 1 \le j \le M. \tag{2}$$

In figure 3c, we show a plot of $dE^{ij}$ in grayscale for $1 \le i \le N$ and for $1 \le j \le M$. The range of the index $i$ translates to the range of the reference thickness as $0 \le h_r \le 4\,\mu$m, and $j$ to $0 \le x \le 1\,$mm. In the plot, black means $dE = 0$ and hence zero color difference, whereas white means the largest color difference. A vertical line at a particular value of $x$ has all possible values of the film thickness at that point; the correct thickness value corresponds to the darkest point. In the case that there are multiple dark points on the same vertical line with insignificant difference between them, thickness determination is not trivial. We note that, however, the film profile is continuous and smooth. Evidently, there are only a few continuous dark lines that can be distinguished without any abrupt change in slope. In figure 3c, we show the candidate profiles in white solid lines (labeled from (i) to (v)). The film thickness profile can be identified by considering the average color difference $\langle dE\rangle$ along each candidate profile $L$:

$$\langle dE\rangle^L = \frac{1}{N_L}\sum_L dE^L, \tag{3}$$

where the sum is taken for all the pixels along the profile and then divide by the number of pixels ($N_L$). In figure 3d, we show $\langle dE\rangle$ for all profiles. The smallest color difference is along profile $(iv)$ for which $\langle dE\rangle^{iv} = 0.038$, whereas the second smallest one is along profile $(iii)$ for which $\langle dE\rangle^{iii} = 0.072$. As a result, we conclude that profile $(iv)$ is the thickness profile of the air film. In figure 3e, we show the computed profile plotted against the profile of the lens used to generate the interference pattern. The difference $\Delta h$ between the two profiles (shown in figure 3f) is within 40 nm.

---


[1] R.W.G. Hunt, *Measuring Colour* (Fountain Press, Kingston - Upon - Thames, UK, 1998).

[2] C. Lin and R.F. Sullivan, IBM J. Research and Development, **16**, 269 (1972).
